# Supplementary material for: Domain-Centered Support for Layout, Tasks, and Specification for Control Flow Graph Visualization
Source: arXiv:2108.03047 source file (2022-09-26)
Supplement: Supplementary file 1 [file appendix.tex]

\section{Overview}

These materials contain more details regarding the literature review
(Sect.~\ref{sec:litreview}), user study
(Sect.~\ref{sec:studydetails}), and our analysis of \textit{CFGConf} using the
Cognitive Dimensions of Notation (Sect.~\ref{sec:cdndetails}). Additional
figures are in Sect.~\ref{sec:extended_examples}.

Data files used in Sect.~IV (Examples) in the main documents can be found at:
\url{https://github.com/hdc-arizona/cfgConf/tree/main/supplementary/example-files}.

\section{Drawing Conventions Literature Review}
\label{sec:litreview}

We sought out figures in conference papers to broaden our understanding of CFG
drawing conventions. We created a list of conferences where CFG drawings might
occur from our collaborators. The conferences are listed below:

\begin{itemize}
  \item International Symposium on Code Generation and Optimization (CGO) (2016 - 2020)
  \item Programming Language Design and Implementation (PLDI) (2019 - 2020)
  \item The International Conference for High Performance Computing,
    Networking, Storage, and Analysis (SC) (2017 - 2019)
\end{itemize}

We viewed all papers published in these conferences, picking out ones which
showed node-linked diagrams. We originally planned to consider three years for
each conference, however we extended our search for CGO and limited for PLDI
based on our successes and failures in finding CFGs in those conferences.

We collected 65 papers with node-link diagrams. From those 65 papers, we found
15 true CFGs (some with added data), 17 CFG-like networks, 11 trees,
and 26 other node-link diagrams. 

We considered a graph "CFG-like" if it also illustrated program flow or
dependencies. These included program dependence graphs, flow and state graphs,
data flow graphs, data dependency graphs, I/O flow graphs, and program graphs.
All other non-tree graphs went into the other category.

When choosing designs, we were most heavily informed by the CFG and CFG-like
drawings. The other graphs showed a wider variance in drawing styles, though
they also tended to follow paradigms such as top-down ordering.

We then coded the diagrams for drawing conventions. The full list of papers
and codes is available as the file
literature\_survey\_drawing\_conventions.xlsx. 

Our codes include layout parameters, such as the general organization of flow
(e.g., top-bottom, left-right), groupings of nodes (enclosure), and alignments
(vertical, horizontal). CFGs displaying the loop layout from CFGExplorer were
given the code ``loopify layout.'' We also noted where labels appeared and
stylistic changes to primitives such as color, texture, shape, borders, and
opacity. 

Due to the small nature of most of these graphs, we were unable to discern
alignment or organization of nodes in a row (or column), which was something
we were expecting to see. Also, only one graph showed elision of nodes.

We noted a few layouts that were coded ``compact'' where we noticed a
trade-off between linear flow and making the figure fit or taking advantage of
white-space. We did not consider implementing these features as we focused on
exploratory analysis use cases rather than journal article concerns.

\section{User Study Details}
\label{sec:studydetails}

The user study can be accessed directly at the following URL:
\url{https://github.com/hdc-arizona/cfgConf/blob/main/user-study-instructions.md}

The participants were first asked to setup \textit{CFGConf} by following the
\texttt{Setup Guide} in the documentation. Setup involved cloning the
\textit{CFGConf} repository, starting the \texttt{http.server}, and creating a
simple two-node drawing and running it as the ``Hello, World'' example. 

The participants were then given the following task prompts:

\textbf{Task 1: } Replicate the drawing below (Fig.~\ref{fig:task1}).
In other words, create a CFGConf JSON file that creates the provided drawing.

\begin{figure}[!ht]
   \centering
   \includegraphics[width=0.2\textwidth]{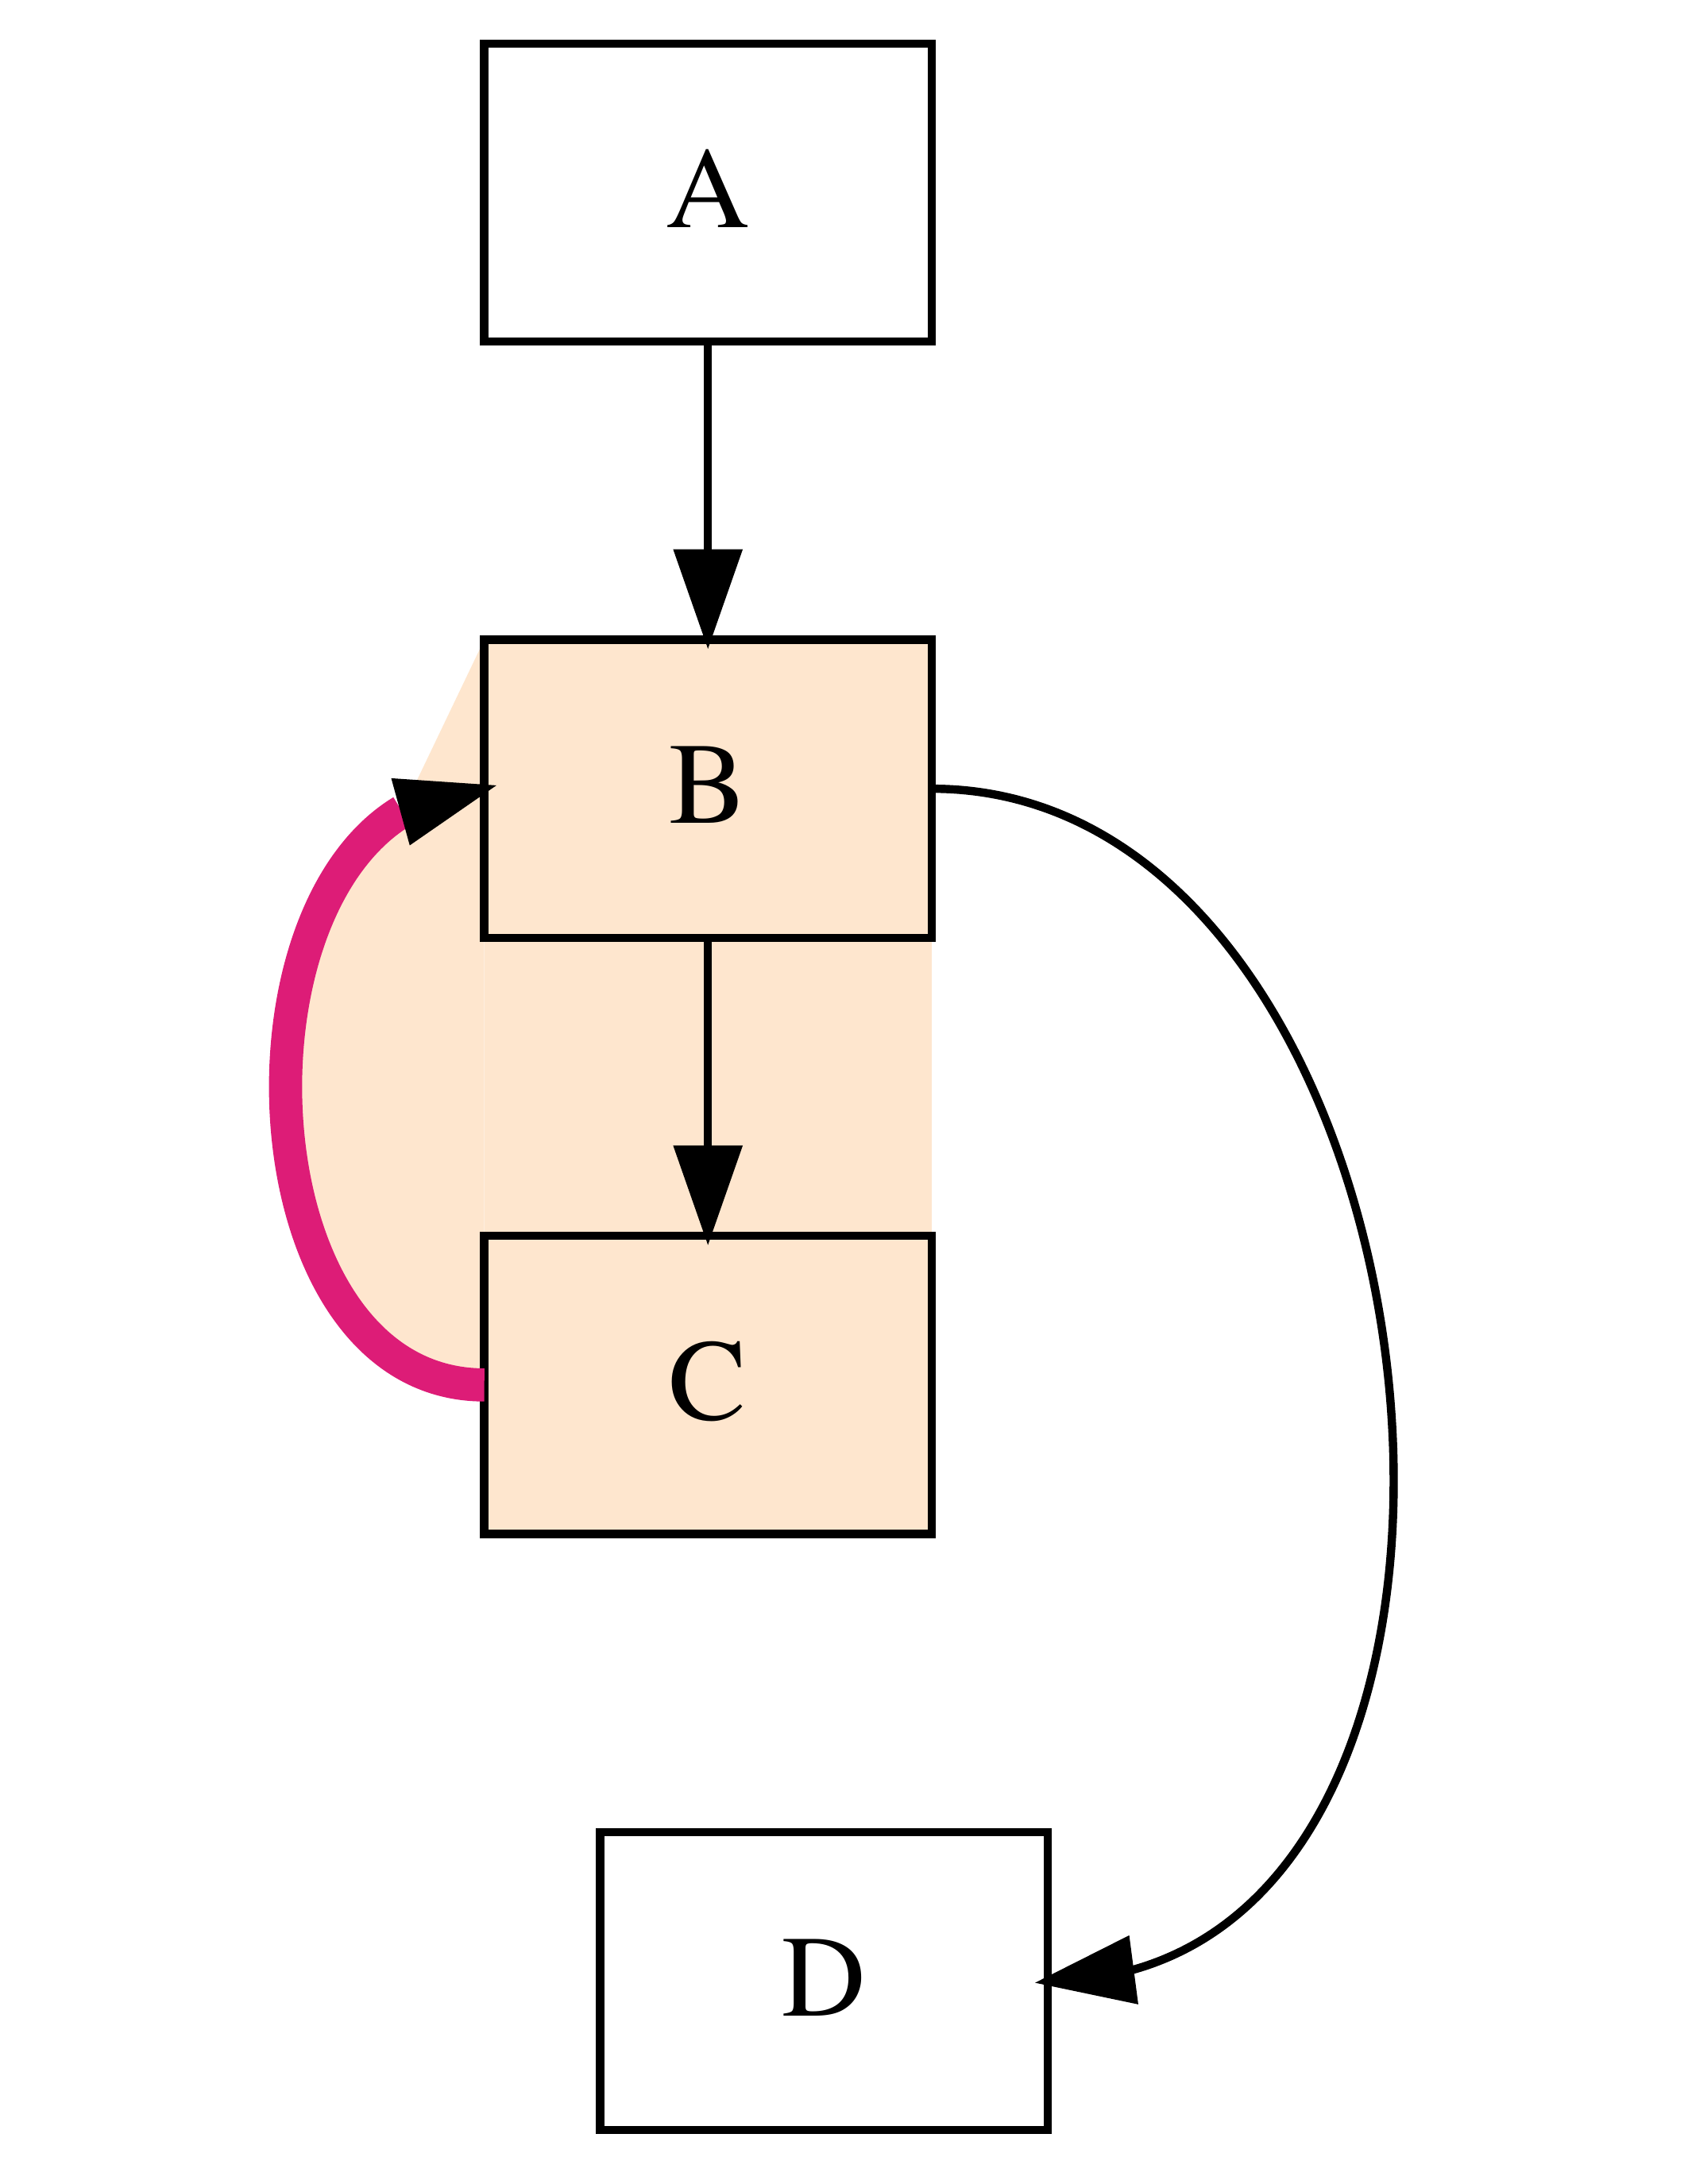}
   \caption{Prompt image for Task1.}
\label{fig:task1}
\end{figure}

\textbf{Task 2.1: } Produce a drawing of the graph from the dot file
\texttt{t2.dot}. Loops inside the graph are provided in the file
\texttt{t2\_loops.json}.

\textbf{Task 2.2: } Compare the resulting drawing from CFGConf to a
drawing produced using dot graphviz on the file \texttt{t2.dot}. Note: These
drawings are expected to appear different. Do not be concerned if they do not
look the same.\\

To produce a pdf file using graphviz, you can run the following command in the
terminal. The drawing \texttt{t2.pdf} will be created in the same directory. 

\begin{center}
    \texttt{dot -Tpdf t2.dot -o t2.pdf}
\end{center}

\textbf{Task 3.1: } Produce a filtered drawing using the graph
specified in \texttt{ltimes.dot}. A dyninst analysis file named
\texttt{ltimes.json} with the functions and loops is also provided.\\

In this drawing, show only the node ids in the boxes, rather than the
disassembly like the previous example.\\

Use the following set of nodes as the starting nodes for filtering:

\begin{center}
\texttt{"B1973", "B1974", "B1978", "B1986", "B1993", "B4052", "B4183", "B4205", "B4206", "B4430"}
\end{center}

The drawn graph should be limited to nodes within \textbf{3 hops} of the above
set and have no more than \textbf{25 nodes} total.

\textbf{Task 3.2: } Turn off the filtering and view the changed output.

\textbf{Task 4: } Produce a filtered drawing using the same graph files
\texttt{ltimes.dot} and \texttt{ltimes.json} with collapsed functions.\\

Specifically, the functions in the filtered graph should be collapsed unless
they contain loops, with the exception of the function
\texttt{\_\_kmpc\_fork\_call}. Ensure \texttt{\_\_kmpc\_fork\_call} is still
drawn.\\

Use the following set of nodes as the starting nodes for filtering:

\begin{center}
\texttt{"B3805", "B4451"}
\end{center}

The survey contained the following open response questions:

\begin{enumerate}
    \item Please add your comments on task 1 e.g., the strategy you used, what worked, what didn't etc.
    \item Please add your comments on task 2 e.g., the strategy you used, what worked, what didn't etc.
    \item Please add your comments on task 3 e.g., the strategy you used, what worked, what didn't etc.
    \item Please add your comments on task 4 e.g., the strategy you used, what worked, what didn't etc.
    \item What, if anything, did you find easy about using CFGConf?
    \item What, if anything, did you find difficult about using CFGConf?
    \item What are the ways in which CFGConf's JSON language and system can be improved?
    \item Do you have scenarios in which you would use CFGConf? If so, please describe.
\end{enumerate}

The participants could upload their \textit{CFGConf} JSON files through the
survey or email them to the lead author. Only the lead author had access to
participant identifying information.

\section{Heuristic Evaluation with CDN}
\label{sec:cdndetails}

The Cognitive Dimensions of Notation (CDN)~\cite{cogdimnotation1989} is a
framework to assess programming languages. Instead of evaluating the
accessibility and notational efficiency of the language using metrics like the
number of lines of code required to generate a drawing, CDN provides a
collection of cognitive dimensions that work as design principles for
languages. As described in Sect.~III of the main document, we assessed
\textit{CFGConf} in light of the cognitive dimensions.  
We describe the cognitive dimensions here and discuss the extent to which
\textit{CFGConf} fulfills them, summarizing our assessment on a scale of Poor,
Fair, Good, Very Good, and Excellent.

\textbf{Abstraction.} Abstraction assesses how well the language
supports defining new terms and concepts to clarify the existing program.
While \textit{CFGConf} provides higher-level abstractions, developed to match
concepts and structures in CFG, it is a specification and not a programming
language. Therefore, it does not support creating new abstractions. This
ability was requested by Participant 3 in user study. Furthermore, in
providing the higher-level abstraction, lower-level details about the layout
algorithm are not directly available in CFGConf. Thus, we describe
\textit{CFGConf}'s fulfillment of Abstraction to be Fair.

\textbf{Closeness of Mapping.} Closeness of mapping assesses how well
the language matches the problem and how users might describe the problem
apart from the notation. CFGConf uses higher-level abstractions such as
\texttt{loops} and \texttt{functions} that match the CFG problem space. The
notation also borrows from existing ones in terms of styling the graphical
elements, support the existing \texttt{dot} format, though there could be some
confusion between \texttt{dot} and \texttt{CSS}. We thus describe CFGConf's
fulfillment of Closeness of Mapping to be Very Good.

\textbf{Consistency.} Consistency assesses how well the language casts
similar actions and features using the same terms. At a low level,
\textit{CFGConf} is consistent in its use of camel-case and using `is' to
denote boolean keys. Styling on nodes and edges uses the same value keywords.
Where possible, \textit{CFGConf} is consistent with other languages, e.g.,
using data formats similar to GraphML and style encodings consistent with
d3js, vega-lite, and \texttt{dot}. We recognize this is a mix of sources, so
we describe \textit{CFGConf}'s fulfillment of Consistency as Very Good.

\textbf{Diffusiveness.} Diffusiveness (alternatively, Terseness)
assesses how concisely the language supports its goals. When separating the
data files (e.g., \texttt{graphFile}, \texttt{structureFile}), the
\textit{CFGConf} specification is generally quite terse. Most of the keys and
objects are not required. However, Participant 2 mentioned \textit{CFGConf}
was verbose. Participant 2 tried copying the data by hand in the second task,
which may have contributed to this assessment. The JSON format for graph
definitions is more diffuse than the \texttt{dot} style. Thus, we consider
\textit{CFGConf}'s diffuseness as Good.

\textbf{Error-Proneness.} Error-proneness assesses how likely users of
the language are to make mistakes or slips. As \textit{CFGConf} is based in
JSON, common slips in JSON, such as missing commas and unmatched quotations or
brackets, are also present in \textit{CFGConf}. Participant 2 in our user
study noted this as a difficulty. As \textit{CFGConf} allows overriding of
style parameters, users could forget which ones contain this information. We
thus describe \textit{CFGConf}'s fulfillment of Error-Proneness to be Good.

\textbf{Hardness of Mental Operations.} Hardness of mental operations
assesses how much mental effort is required to produce the language.
\textit{CFGConf} is declarative in nature, built on the widely used JSON
format, so we expect most operations to not be difficult. However, the
non-required parameters in filtering and function collapsing may need
additional thought, especially for users unfamiliar with these concepts. We
thus describe \textit{CFGConf}'s fulfillment of Hardness of Mental Operations
as Good.

\textbf{Hidden Dependencies.} Hidden dependencies refer to dependencies
between parts of the language, where changing one may lead to unintended
effects or require previous unknown changes. These dependencies can compound,
making it difficult to change as the specification gets longer.

Generally, related specifications in \textit{CFGConf} are within the same JSON
object, and thus apparent. We do set several defaults to support
diffuseness/terseness, but these do not affect the other parts of
specification. The one exception is style overrides, which move from the
\texttt{rendering} section to the \texttt{data} section, which was a trade off
made for both terseness and consistency and compatibility with \texttt{dot}. 

All changes, even style-related ones, have the possibility of affecting the
final graph layout. Given the complicated optimization done in the underlying
algorithm, the dependency between these declarations and the final
visualization is unknowable. Users understand in general what changes will
happen, but cannot predict the final layout. Therefore, we describe
\textit{CFGConf}'s handling of hidden dependencies as Good.

\textbf{Premature Commitment.} Premature commitment assesses how
flexible the language is to working on its parts and making decisions about
the final specification in any order. \textit{CFGConf} is declarative and
modularized. As long as their names for data and IDs do not change, they
should be able to come to the same specification regardless of the order they
write it. Thus, we describe \textit{CFGConf} as Excellent in terms of
Premature Commitment.

\textbf{Progressive Evaluation.} Progressive evaluation assesses
whether the language permits checking incomplete work, i.e., running the
program when it is not yet fully written. \textit{CFGConf} applies default
values where drawing parameters are unspecified. Users can refine their
drawing by setting more parameters. Thus, we describe \textit{CFGConf} as
Excellent in terms of Progressive Evaluation.

\textbf{Role-Expressiveness.} Role-expressiveness assesses how easy or
difficult it is to understand each part of the language, both in reading it
and producing it. \textit{CFGConf} has three top-level keywords for
\texttt{data}, \texttt{rendering}, and \texttt{filtering} respectively. The
first two are further broken down according to their semantic application,
e.g., \texttt{nodes}, \texttt{edges}, \texttt{loops}, and \texttt{functions}.
We thus describe \textit{CFGConf}'s Role-Expressiveness as Excellent.

\textbf{Secondary Notation.} Secondary notation refers to the ability
to annotate the program or add additional information that is not part of the
language. \textit{CFGConf} is based on JSON, which does not have a comment
capability. As \textit{CFGConf} is robust to unrecognized keys, auxiliary
information, including comments, can be specified as a key-value pair, but
this is not ideal. Thus, we describe \textit{CFGConf}'s support for Secondary
Notation as Fair.

\textbf{Visibility.} Visibility assesses the ease of identifying,
finding, and comparing parts of the language. \textit{CFGConf} is JSON-based
and can be written in a single file. When the data is large, it can be placed
in a separate file, with the remaining keywords likely fitting in a single
screen, though this could separate style overrides from global style options.
Most of the keywords are semantically meaningful, thus helping with search and
comparison. We thus describe \textit{CFGConf}'s Visibility as Very Good.

\textbf{Viscosity.} Viscosity assesses how difficult it is to make
changes in the languages, including whether changing one part requires more
changes in other parts. The modular design of \textit{CFGConf} allows users to
make changes within a single top-level JSON object. The most difficult change
would be changing the ID of a node, edge, loop, or function when it is
referenced elsewhere. \textit{CFGConf} recognized a separate \texttt{label}
keyword to discourage these changes.  We thus describe \textit{CFGConf}'s
Viscosity as Very Good.

\section{\textit{CFGConf} Rendering Style Example}
\label{sec:extended_examples}

\begin{figure}[!hb]
\centering
\includegraphics[width=0.35\textwidth]{imgs/singlefile_rendering_json.pdf}
\caption{Specification with global style parameters, resulting in~\autoref{fig:singlefile_rendering}.} \label{fig:singlefile_rendering_json}
\end{figure}

\autoref{fig:singlefile_rendering} shows a CFG styled globally with a
different node color and shape based on the specification in
\autoref{fig:singlefile_rendering_json}. Function nodes are grouped together
and enclosed with rectangular boundaries.

\begin{figure*}[htb]
\centering
\includegraphics[width=0.7\textwidth]{imgs/singlefile_rendering_rotated.pdf}
\caption{A CFG styled globally with diamond shape nodes with a green background. Rectangular boxes group nodes belonging to the same function. This drawing has been rotated to better utilize the aspect ratio of this format.} \label{fig:singlefile_rendering}
\end{figure*}
